# Supplementary material for: Finding Birkhoff Averages via Adaptive Filtering
Source: arXiv:2403.19003 source file (2024-03-27)
Supplement: Supplementary file 2 [file integrated_convergence.tex]

\section{Integrated Sequence Bound}
\begin{lemma}
    Let $\{a_n\}$ be a sequence with the bound $\abs{a_n} < C n^{-M}$. Then,
    \begin{equation*}
        \abs{\sum_{n>N} a_n} \leq \sum_{n>N}\abs{a_n} \leq C_2 N^{-M+1}.
    \end{equation*}
\end{lemma}
\begin{proof}
    The first part is obvious. The second part is performed by the integral test.
    \begin{align*}
        \sum_{n > N} \abs{a_n} \leq C \sum_{n > N} n^{-M} \leq C \int_{N}^\infty x^{-M} \dif x = \frac{C}{M-1} N^{-M+1}.
    \end{align*}
\end{proof}

\begin{lemma}
\label{lemma:Diophantine}
    Let $\omegabf$ satisfy the Diophantine condition
    \begin{equation*}
        \abs{\nbf \cdot \omega - m} \geq \frac{C}{\abs{\nbf}^{\nu}}.
    \end{equation*}
    Then, 
    \begin{equation*}
        \abs{1-e^{2\pi i \nbf \cdot \omegabf}} > \frac{2C}{\abs{\nbf}^{\nu}}.
    \end{equation*}
\end{lemma}
\begin{proof}
    First, we note that 
    \begin{equation*}
        \abs{1-e^{2\pi i \nbf \cdot \omegabf}} = \abs{\sin\left(\pi (\nbf \cdot \omegabf - m) \right)},
    \end{equation*}
    where we assume $m\in \Zbb$ is chosen so that $\abs{\nbf \cdot \omegabf - m}\leq 1/2$. On this domain, the function 
    \begin{equation*}
        \abs{\sin\left(\pi (\nbf \cdot \omegabf - m) \right)} > 2\abs{\nbf \cdot \omegabf - m} \geq \frac{2C}{\abs{\nbf}^{\nu}}.
    \end{equation*}
\end{proof}

\begin{theorem}
    Under Hypotheses \ref{setting} with $M > \nu + d$, the unweighted Birkhoff average of invariant circles converges as $\Ocal(T^{-1})$. 
\end{theorem}
\begin{proof}
    The unweighted Birkhoff average is given by
    \begin{align*}
        \BA_T[\obs](\xbf) = \sum_{t = 0}^{T-1} \frac{1}{T} (\obs \circ \zbf)(\thetabf + \omegabf).
    \end{align*}
    Using the Fourier series representation of $\obs \circ \zbf$, we have
    \begin{align*}
        \BA_T[\obs](\xbf) - h_0 &= \frac{1}{T} \sum_{\nbf \in\Zbb^d \backslash\{0\}} \obsT_{\nbf}  \sum_{t=0}^{T-1}e^{2\pi i t \nbf \cdot \omegabf},\\
        &= \frac{1}{T} \sum_{\nbf \in\Zbb^d \backslash\{0\}} \obsT_{\nbf} \frac{e^{-2\pi i \nbf \cdot \omegabf}-e^{2\pi i (T-1)\nbf \cdot \omegabf}}{1-e^{2\pi i \nbf \cdot \omegabf}}.
    \end{align*}
    Using the continuity bounds $\abs{\obsT_{\nbf}}<C_h \abs{\nbf}^{-M}$ and Lemma \ref{lemma:Diophantine}, we have
    \begin{align*}
        \abs{\BA_T[\obs](\xbf) - h_0} & \leq \frac{C_h}{C T} \sum_{\nbf \in\Zbb^d \backslash\{0\}} \obsT_{\nbf} \abs{\nbf}^{-M + \nu}.
    \end{align*}
    For the convergence of this sum, we require $-M+\nu < -d$, or $M > d+\nu$.
\end{proof}
