# Supplementary material for: Finding Birkhoff Averages via Adaptive Filtering
Source: arXiv:2403.19003 source file (2024-03-27)
Supplement: Supplementary file 3 [file RealAnalyticStuff.tex]

Just to make sure I still know how to do analysis...
\begin{lemma}
    A real analytic function $f\in C^{\omega}(\Tbb_\rho)$ with $\norm{f}_\rho < \infty$ has Fourier coefficients that obey
    \begin{equation*}
        \abs{f_n} \leq \norm{f}_\rho e^{-n\rho}.
    \end{equation*}
\end{lemma}
\begin{proof}
    A Fourier coefficient of $f$ can be computed via
    \begin{equation*}
        f_n = \frac{1}{2\pi}\int_{\Tbb} f(\theta) e^{- i n \theta} \dif \theta,
    \end{equation*}
    where WLOG we assume $n>0$. 
    For any $\rho_* < \rho$, by deforming the integration contour vertically, we have
    \begin{equation*}
        f_n = \frac{e^{-n\rho_*}}{2\pi}\int_{\Tbb} f(\theta - i \rho_*) e^{-i n \theta} \dif \theta.
    \end{equation*}
    This can be bounded by
    \begin{equation*}
        \abs{f_n} = \norm{f}_{\rho} e^{- n\rho_*}.
    \end{equation*}
    Now, we have that
    \begin{equation*}
        \limsup_{\rho_* \to \rho} \abs{f_n} \leq \limsup_{\rho_*\to\rho} \norm{f}_{\rho} e^{-n\rho_*} = \norm{f}_{\rho} e^{-n\rho}.
    \end{equation*}
\end{proof}

\begin{lemma}
    Furthermore, we have 
    \begin{equation*}
        \sum_{\abs{n} > N} \abs{f_n} < C e^{-N\rho}.
    \end{equation*}
\end{lemma}
\begin{proof}
    We have
    \begin{align*}
        \sum_{\abs{n} > N} \abs{f_n} &< 2 \norm{f}_{\rho} \sum_{n > N}\left(e^{-\rho}\right)^n,\\
        &= \frac{2 \norm{f}_{\rho} e^{-\rho{N+1}}}{1-e^{-\rho}}
    \end{align*}
\end{proof}
