# Supplementary material for: Finding Birkhoff Averages via Adaptive Filtering
Source: arXiv:2403.19003 source file (2024-03-27)
Supplement: Supplementary file 4 [file fourier_gaps.tex]

\section{Distribution of gaps in a Fourier series}
\mr{A better version of this must exist somewhere...}
\begin{lemma}
\label{lemma:Fourier-gaps}
    Let $\dobsT$ be a function with a bound on the Fourier coefficients of the form $\abs{\dobsT_n} < C n^{-M}$ for some $M\geq 1$. Then for every $\epsilon > 0$, there exists a gap $\delta$ between values of $\abs{\dobsT_n}$ with the lower bound
    \begin{equation*}
        \delta > C_2 \epsilon^{1 + 1/M}.
    \end{equation*}
\end{lemma}
\begin{proof}
    First, consider the value of $N$ such that $n > N$ implies $\abs{\dobsT_n} < \epsilon/2$. This is given by
    \begin{equation*}
        N = \left( \frac{\epsilon}{2 C}\right)^{-1/M}.
    \end{equation*}
    This means that at most $N$ coefficients can be within the region $(\epsilon/2, \epsilon]$, guaranteeing a gap of size at least $\epsilon/(2N+2)$. This gives our theorem
\end{proof}
