# Supplementary material for: Finding Birkhoff Averages via Adaptive Filtering
Source: arXiv:2403.19003 source file (2024-03-27)
Supplement: Supplementary file 5 [file symmetric_eigenvalue_perturbation_theorems.tex]

\section{Eigenvalue Problem Perturbation Theorems}
Here, we quote three eigenvalue perturbation theorems used in the proofs herein. For the following theorems, denote $\mathcal L(A)$ as the set of eigenvalues of a matrix $A$. All theorems are taken from Stewart and Sun\cite{Stewart1990} (SS).

\begin{theorem}[Gershgorin, SS Thm.~2.2.1]
\label{thm:gershgorin}
For $A \in \Cbb^{n\times n}$ let
\begin{equation*}
    R_i = \sum_{j \neq i} \abs{a_{ij}}
\end{equation*}
and
\begin{equation*}
    \mathcal G_i(A) = \left\{z \in \Cbb \mid \abs{z-a_{ii}} \leq a_i \right\}.
\end{equation*}
Then 
\begin{equation*}
    \mathcal L (A) \subset \bigcup_{i=1}^n \mathcal G_i(A).
\end{equation*}
\end{theorem}

\begin{theorem}[Weyl's, SS Cor.~4.4.9] 
\label{thm:Weyl}
Let $A$ and $E$ be symmetric matrices with eigenvalues $\{\sigma_i\}$ and $\{\epsilon_i\}$ respectively, ordered so that $\sigma_i \geq \sigma_{i+1}$ and $\epsilon_i \geq \epsilon_{i+1}$.  Then, for $i = 1, \dots, n$, the eigenvalues $\tilde{\sigma}_i$ of $\tilde{A} = A + E$ satisfy
\begin{equation*}
    \tilde{\sigma}_i \in [\sigma_i + \epsilon_n, \sigma_i + \epsilon_1].
\end{equation*}
\end{theorem}

\begin{theorem}[Davis-Kahan $\sin(\Theta)$, SS Thm.~5.3.4, 5.3.6, 5.3.8]
\label{thm:DavisKahan}
    Let $A$ be a Hermitian matrix with spectral resolution
    \begin{equation*}
        \begin{pmatrix}
            X_1^* \\ X_2^*
        \end{pmatrix}
        A
        \begin{pmatrix}
            X_1 & X_2
        \end{pmatrix}
        = 
        \Diag(L_1, L_2),
    \end{equation*}
    where $\begin{pmatrix}
        X_1 & X_2
    \end{pmatrix}$ is unitary with $X_1 \in \Cbb^{n\times k}$. Let $Z \in \Cbb^{n\times k}$, and $M\in \Cbb^{k\times k}$ be Hermitian, and
    \begin{equation*}
        R = A Z - Z M.
    \end{equation*}
    Suppose that 
    \begin{equation*}
        \mathcal L (M) \subset [\alpha, \beta]
    \end{equation*}
    and that for some $\delta > 0$
    \begin{equation*}
        \mathcal L (L_2) \subset \mathbb{R} \backslash [\alpha-\delta, \beta + \delta].
    \end{equation*}
    Then for any unitarially invariant norm
    \begin{equation*}
        \norm{\sin \Theta[\Rcal(X_1), \Rcal(Z)]} \leq \frac{\norm{R}}{\delta \inf_2(Z)},
    \end{equation*}
    where $\inf_2(Z)$ is the smallest singular value of $Z$. 
\end{theorem}
