# Supplementary material for: Finding Birkhoff Averages via Adaptive Filtering
Source: arXiv:2403.19003 source file (2024-03-27)
Supplement: Supplementary file 6 [file base_polynomial.tex]

\section{The Base Polynomial}
\label{subsec:45}

In the introduction, we mentioned that not only do we need control over the normal matrix, but also over the filter that we perturb around. For this, we will use the following polynomial:
\begin{lemma}
\label{lemma:refpolybound}
    Let $0 < \omega \leq 1$ have a sequence of continued fractions approximants with $\{a_n / L_n \}$. For any $n \geq 1$ and $\alpha < 1/4$, define the polynomial
    \begin{equation}
    \label{eq:refpoly}
        \refpoly(z) = \left(\prod_{j = 1}^{\floor{\alpha p L_{n}}}\frac{(z - \lambda_j)(z - \lambda_{-j})}{(1 - \lambda_j)(1 - \lambda_{-j})}\right)
        \left(\prod_{j = \floor{\alpha p L_{n}}+1}^{\floor{{p L_{n}}/{2}}}\frac{(z - \tilde \lambda_j)(z - \tilde \lambda_{-j})}{(1 - \tilde \lambda_j)(1 - \tilde \lambda_{-j})}\right)
    \end{equation}
    where for $0 \leq \ell < p$ and $j\geq 0$
    \begin{equation*}
        \tilde \lambda_{j p + \ell} = e^{2 \pi i (j a_n/L_n + \ell)/p}.
    \end{equation*}
    Then, the polynomial obeys the bound $\abs{\refpoly(z)} \leq C_\alpha$ for $\abs{z} \leq 1$ and $C_\alpha > 1$, where $C_\alpha$ is independent of $\omega$ and $m$.
\end{lemma}
\begin{proof}
    The proof consists of comparing the polynomial above to the polynomial with equispaced nodes 
    \begin{equation*}
        Q_{\alpha, \omega, n, p}(z) = \prod_{j = 1}^{\floor{{L_{n}}/{2}}}\frac{(z - \tilde \lambda_j)(z - \tilde \lambda_{-j})}{(1 - \tilde \lambda_j)(1 - \tilde \lambda_{-j})}.
    \end{equation*}
    We begin by assuming $L_n$ is odd. In this case, the polynomial coefficients of $Q_{\alpha, \omega, n, p}$ can be thought of as a column of the inverse discrete Fourier transform. This is because we have $Q(1) = 1$ and $Q(\tilde \lambda_j) = 0$ for $1 \leq \abs{j} \leq \floor{\nicefrac{L_n}{2}}$ So, $Q_{\alpha, \omega, n, p}$ is simply the interpolation of a unit vector that is nonzero at $1$, i.e.~$\qbf = F^{-1} \ebf_0$ where $\qbf$ are the polynomial coefficients and $F$ is the mapping from Fourier coefficients to values at equispaced nodes.

    The problem of how Fourier interpolation changes when the nodes are perturbed is addressed in \cite{yu2023}. In this paper, Yu and Townsend prove an analogue to the Kadec-$1/4$ theorem \cite{kadets1964} from sampling theory, which states that as long as the locations of Fourier nodes does not move a length farther than $\alpha/4$ from the equispaced grid, the mapping from these Fourier space to these modes $\tilde{F}$ does not differ too much in norm from the standard mapping, i.e.
    \begin{equation*}
        \norm{\tilde F} \leq (1 + \phi_\alpha)\norm{F}_2,
    \end{equation*}
    where $\norm{F} = L_n$ and $\phi_\alpha = 1 - \cos \pi \alpha + \sin \pi \alpha$. Additionally, via Weyl's inequality we have
    \begin{equation*}
        \norm{\tilde F^{-1}}_2 \leq \frac{1}{(1 - \phi_\alpha) \norm F}_2.
    \end{equation*}
    
    We can apply these identities to our problem. In particular, we note that continued fraction approximations obey the bound
    \begin{equation*}
        \abs{\omega - \frac{a_n}{L_n}} < \frac{1}{L_n^2}.
    \end{equation*}
    Using this, we find that $\abs{\lambda_j - \tilde \lambda_j} < \alpha \pi / L_n$ for $\abs{j} < \floor{\alpha L_n}$, obeying the hypothesis for the $1/4$ theorem. Hence, the coefficients of $\refpoly$ 
    \begin{equation*}
        \norm{\pbf_{\alpha, \omega, n}}_2 = \norm{\tilde F^{-1} \ebf_0}_2 \leq \frac{1}{(1-\phi_\alpha)\sqrt{L_n}}. 
    \end{equation*}
    The bound directly follows from the above inequality. 
\end{proof}
The polynomials $\refpoly$ also obeys a bound on its derivatives. In Lemma \ref{lemma:refpolyderivbound}, we show that general polynomials with perturbed roots have lower bounds on their derivatives. We state the result for our polynomial as a corollary:
\begin{corollary}
\label{corollary:refpolyderivbound}
    Let $\alpha < 1/4$. The derivative of $\refpoly(z)$ at each root $\lambda$ obeys
    \begin{equation*}
        \abs{\refpoly'(\lambda)} \geq C N^{-4\alpha}
    \end{equation*}
    for some constant $C$.
\end{corollary}
\begin{proof}
    See Lemma \ref{lemma:refpolyderivbound} and use the bounds from the proof of Lemma \ref{lemma:refpolybound}.
\end{proof}
