# Supplementary material for: Finding Birkhoff Averages via Adaptive Filtering
Source: arXiv:2403.19003 source file (2024-03-27)
Supplement: Supplementary file 12 [file polynomial_derivative_bound.tex]

\section{Bounding the polynomial derivative}
\begin{lemma}
\label{lemma:refpolyderivbound}
    Let
    \begin{equation*}
        p(z) = \prod_{\substack{0 \leq n < N \\ n \neq 0}} \frac{z - \lambda_n}{\lambda_0 - \lambda_n}, \qquad \lambda_n = e^{2\pi i (n + \alpha_n)/N},
    \end{equation*}
    where $\alpha_n < \alpha$. If $\alpha < 1/4$, the derivative of $p$ at the roots $\lambda_m$ obeys
    \begin{equation*}
        \abs{p'(\lambda_m)} \geq C N^{-4\alpha}, \qquad 1 \leq m < N
    \end{equation*}
    for some constant $C$.
\end{lemma}
\begin{proof}
    Evaluating $p'$ at a node, we have
    \begin{equation*}
        p'(\lambda_m) = \frac{1}{\lambda_0 - \lambda_m} \prod_{\substack{0 \leq n < N \\ n \neq 0, m}}\frac{\lambda_m - \lambda_n}{\lambda_0 - \lambda_n}.
    \end{equation*}
    We can reorder the product numerator so that
    \begin{equation*}
        p'(\lambda_m) = \frac{1}{\lambda_0 - \lambda_m} \prod_{\substack{0 \leq n < N \\ n \neq 0, m}}\frac{\lambda_m - \lambda_{m - n}}{\lambda_0 - \lambda_n},
    \end{equation*}
    where we identify $\lambda_n = \lambda_{n-N}$. Focusing on the term inside the product, we have
    \begin{equation*}
        \lambda_m - \lambda_n = 2 i e^{\pi i (m + n +\alpha_m + \alpha_n)/N} \sin\left(\pi \frac{m - n + \alpha_m - \alpha_n}{N} \right),
    \end{equation*}
    so
    \begin{equation*}
        \frac{\lambda_m - \lambda_{m-n}}{\lambda_0 - \lambda_n} = - e^{\pi i (\alpha_m + \alpha_{m-n} - \alpha_0 - \alpha_n)} \frac{\sin\left(\pi (n + \alpha_m - \alpha_{m-n})/N \right)}{\sin\left(\pi (n + \alpha_n - \alpha_{0})/N \right)},
    \end{equation*}
    and
    \begin{align*}
        \log \abs{p'(\lambda_m)} =& \log \abs{\frac{1}{\lambda_0 - \lambda_m} } + \sum_{\substack{0 \leq n < N \\ n \neq 0, m}} \log \left(\frac{\sin\left(\pi (n + \alpha_m - \alpha_{m-n})/N \right)}{\sin\left(\pi (n + \alpha_n - \alpha_{0})/N \right)}\right), \\
        =& \ C + \sum_{\substack{0 \leq n < \floor{(N-1)/2} \\ n \neq 0, m}}\log \left(\frac{\sin\left(\pi (n + \alpha_m - \alpha)/N \right)}{\sin\left(\pi (n - \alpha_{0} + \alpha )/N \right)}\right) \\
        &+\sum_{\substack{\ceil{(N-1)/2 + 1} \leq n < N \\ n \neq 0, m}}\log \left(\frac{\sin\left(\pi (n + \alpha_m + \alpha)/N \right)}{\sin\left(\pi (n - \alpha_{0} - \alpha )/N \right)}\right),
    \end{align*}
    where $C$ is a constant that includes the the leading term as well as the factor contributed by $n=N/2$ when $N$ is even, which are both bounded from below. Now, for $0 \leq n < \floor{(N-1)/2}$, we have
    \begin{equation*}
        \sin\left(\frac{\pi(n + \alpha_m - \alpha)}{N}\right) 
        \geq 
        \sin\left( \frac{\pi (n - \alpha_0 + \alpha)}{N}\right) 
        - \frac{\pi (2 \alpha - \alpha_0 - \alpha_m)}{N}
        \cos\left(\frac{\pi(n + \alpha_m - \alpha)}{N}\right).
    \end{equation*}
    So,
    \begin{align*}
        \sum_{\substack{0 \leq n < \floor{(N-1)/2} \\ n \neq 0, m}} &\log \left(\frac{\sin\left(\pi (n + \alpha_m - \alpha)/N \right)}{\sin\left(\pi (n - \alpha_{0} + \alpha )/N \right)}\right)
        \geq \\ & \geq
        \sum_{\substack{1 \leq n < \floor{(N-1)/2}}} \log \left( 1 - \frac{\pi (2 \alpha - \alpha_0 - \alpha_m)}{N} \frac{\cos\left(\pi(n + \alpha_m - \alpha)/N\right)}{\sin\left(\pi (n - \alpha_{0} + \alpha )/N \right)}\right),\\
        & \geq 
        \sum_{\substack{1 \leq n < \floor{(N-1)/2}}} \log \left( 1 - \frac{\pi (2 \alpha - \alpha_0 - \alpha_m)}{N} \cot\left(\pi (n - \alpha_{0} + \alpha )/N \right)\right), \\
        & \geq
        \sum_{\substack{1 \leq n < \floor{(N-1)/2}}} \log \left( 1 - \frac{2 \alpha - \alpha_0 - \alpha_m}{n - \alpha_{0} + \alpha} \right), \\
        & \geq -(2\alpha - \alpha_0 - \alpha_m) \sum_{\substack{1 \leq n < \floor{(N-1)/2}}} \frac{1}{n - \alpha_0 + \alpha}, \\
        % & \geq -\frac{(2 \alpha - \alpha_0 - \alpha_m)(1 + 2 \alpha)}{1-2\alpha} \sum_{\substack{1 \leq n < \floor{(N-1)/2}}} \frac{1}{n - \alpha_{0} + \alpha}, \\
        & \geq  -(2\alpha - \alpha_0 - \alpha_m) \left(\frac{1}{1-\alpha_0 + \alpha} + \int_{1-\alpha_0 + \alpha}^{N/2} \frac{1}{x} \dif x \right), \\
        & =  -(2\alpha - \alpha_0 - \alpha_m)\left(\frac{1}{1-\alpha_0 + \alpha} - \log(1 - \alpha_0 + \alpha) - \log 2 + \log(N) \right), \\
        & \geq -(2\alpha - \alpha_0 - \alpha_m) \log N + C,
    \end{align*}
    where we used $\alpha < 1/4$ for the logarithm to have a valid domain and the facts that $1/x \geq \cot x$ for $0 < x \leq \pi/2$ and $\log(1 - y) \geq -y/(1-y)$ for $0 \leq y < 1$. By symmetry, we similarly have
    \begin{align*}
        \sum_{\substack{\ceil{(N-1)/2 + 1} \leq n < N \\ n \neq 0, m}}\log \left(\frac{\sin\left(\pi (n + \alpha_m + \alpha)/N \right)}{\sin\left(\pi (n - \alpha_{0} - \alpha )/N \right)}\right) \geq -(2\alpha + \alpha_0 + \alpha_m) \log N + C,
    \end{align*}
    In total, we find
    \begin{align*}
        \log \abs{p'(\lambda_m)} \geq - 4 \alpha \log N + C,
    \end{align*}
    so
    \begin{align*}
        \abs{p'(\lambda_m)} \geq C N^{- 4 \alpha }
    \end{align*}
\end{proof}
